# Supplementary material for: MoLAE: Mixture of Latent Experts for Parameter-Efficient Language Models
Source: arXiv:2503.23100 source file (2025-05-25)
Supplement: Supplementary file 1 [file appendix2.tex]

% \section{Transformation from MoE to MoLAE} \label{sec:appendix2}

% This section presents our empirical analysis of transforming standard MoE architectures into their corresponding MoLAE counterparts. We specifically investigate the Qwen1.5-MoE-A2.7B model and systematically examine the impact of varying the latent space configuration parameter $k$ on model performance.

% As established in Section \ref{sec:mole_structure}, the parameter $k$ in MoLAE architecture represents a critical hyperparameter that controls the trade-off between parameter efficiency and model expressivity. We evaluate three distinct configurations of $k \in \{1, 10, 20, 30, 60\}$, where:
% \begin{itemize}
% \item $k=1$ corresponds to the original MoE architecture (baseline)
% \item $k=10, 20$ represent a balanced MoLAE configuration with multiple latent spaces
% \item $k=30, 60$ represent the extreme case with only one and two shared latent spaces respectively.
% \end{itemize}

% For consistent evaluation with Section \ref{sec:appendix1}, we assess model performance on three established benchmarks: MMLU (reasoning), GSM8K (mathematical reasoning), and Wikitext-2 (language modeling perplexity).

% Table \ref{table:5} presents the comparative performance across different MoLAE configurations.

% \begin{table}[htbp]
% \begin{center}
% \begin{tabular}{c | c c c}
% \toprule
% \textbf{Number of experts per latent} ($k$) & \textbf{GSM8K} (\%) $\uparrow$ & \textbf{MMLU} (\%) $\uparrow$ & \textbf{Wikitext-2 PPL} $\downarrow$ \\ 
% \midrule
% $1$ (Original MoE) & \textbf{60.1} & \textbf{61.0} & \textbf{9.49} \\
% $10$ & 59.4 & 60.0 & 9.74 \\
% $20$ & 52.8 & 59.0 & 10.15 \\
% $30$ & 19.5 & 48.6 & 12.11 \\
% $60$ & 14.3 & 40.1 & 25.97 \\
% \bottomrule
% \end{tabular}
% \vspace{1ex}
% \caption{Performance comparison of Qwen1.5-MoE-A2.7B with varying MoLAE configurations. The balanced configuration ($k=10$) maintains near-parity with the original model while achieving significant parameter reduction. The single latent space configuration ($k=60$) demonstrates substantial performance degradation.}
% \label{table:5}
% \end{center}
% \end{table}

% The results demonstrate a clear relationship between latent space configuration and model performance. The balanced MoLAE configuration ($k=10$) achieves comparable performance to the original MoE architecture, with only marginal degradation across all benchmarks: a 0.7 percentage point decrease on GSM8K, 1.0 percentage point decrease on MMLU, and 2.6\% increase in perplexity on Wikitext-2. This configuration successfully reduces parameter count while preserving most of the model's capabilities.

% In contrast, the extreme configuration ($k=60$) with a single shared latent space per FFN layer exhibits catastrophic performance degradation: a 45.8 percentage point decrease on GSM8K, 20.9 percentage point decrease on MMLU, and 173.7\% increase in perplexity. This dramatic performance collapse empirically validates our theoretical analysis that multiple latent spaces are necessary to preserve the expressive capacity of the original MoE architecture.

% These findings provide compelling evidence that the MoLAE architecture, when properly configured with an appropriate number of latent spaces, can achieve substantial parameter efficiency while maintaining competitive performance. Furthermore, they establish clear boundaries for the practical application of latent space factorization in expert-based neural architectures.
